# Supplementary material for: Superconductivity coexisting with ferromagnetism in a quasi-one dimensional non-centrosymmetric (TaSe$_4$)$_3$I
Source: arXiv:2111.14525 ancillary file (2021-11-30)
Supplement: Supplementary file 1 [file Supplementary_Information.pdf]

# Supplementary Information

## Superconductivity coexisting with ferromagnetism in quasi-one dimensional non-centrosymmetric $(TaSe_4)_3I$

Arnab Bera, Sirshendu Gayen, Suchanda Mondal, Riju Pal, Buddhadeb Pal, Aastha Vasdev, Sandeep Howlader, Manish Jana, Tanmay Maiti, Rafikul Ali Saha, Biswajit Das, Biswarup Satpati, Atindra Nath Pal*, Prabhat Mandal*, Goutam Sheet*, and Mintu Mondal

---

## Section S1: Crystal growth & characterization of non-centrosymmetric phase of quasi-one-dimensional material, $(TaSe_4)_3I$

The single crystals of non-centrosymmetric phase of $(TaSe_4)_3I$ (named as n-TSI phase) compound were grown by chemical vapor transport (CVT) method. The stoichiometric mixture of the ingredient elements was taken in powder form in a quartz tube and vacuum sealed before it was placed in a two-zone furnace maintained at $500^0$C and $400^0$C for one week. The crystals grow like needles along random directions in the quartz tube. After cooling down the tube to room temperature, the crystals (silver/grey in color) were collected as a lump of fibre wool by

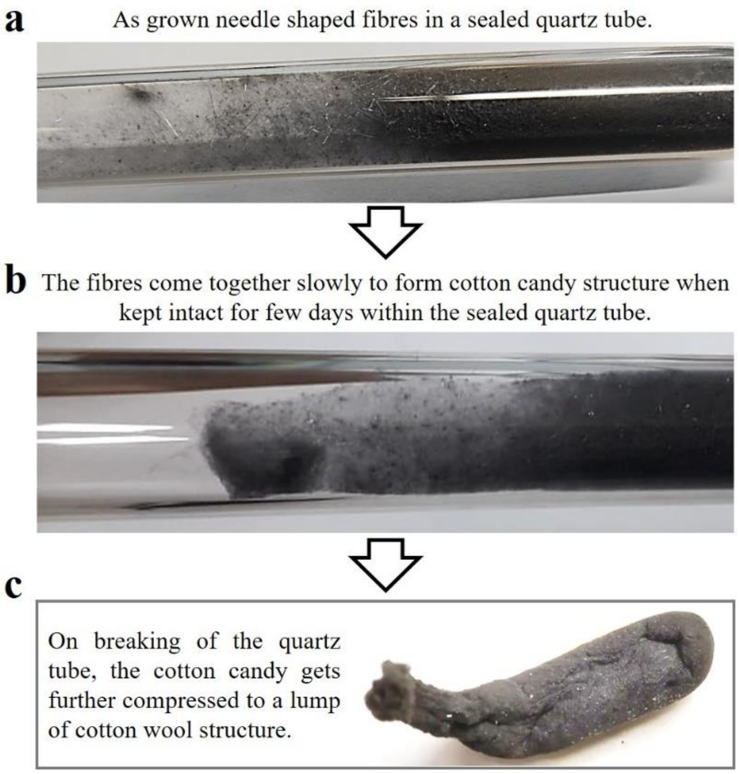


***Figure S1.*** *Schematic showing physical changes of n-TSI occurred with time after growth.*

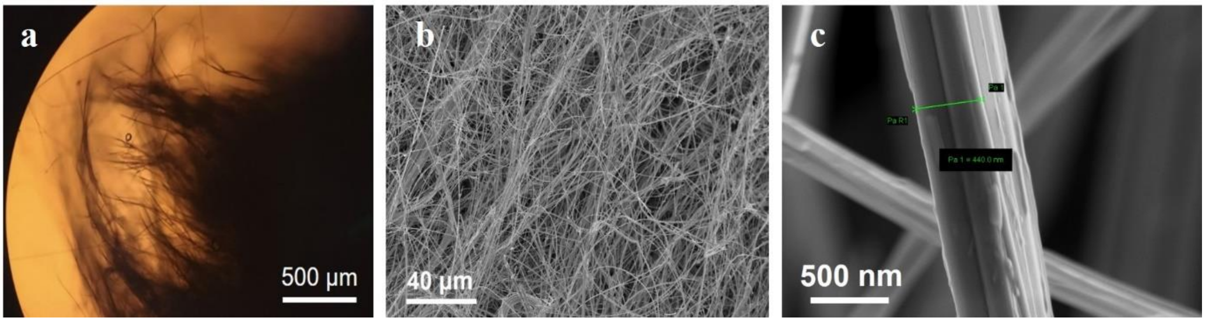


***Figure S2.*** *(a) Image of n-TSI fibres under optical microscope. (b-c) Scanning electron microscopy (SEM) images.*

breaking the quartz tube in air at room temperature (300K). The material is stable under ambient condition. It may be mentioned here that we observed some physical changes of the single crystals with time after the sample growth as shown in Figure S1. (a-c). Such interesting property is possibly related to a large thermo-electric property of the material. Although it is a metal, a small local temperature gradient possibly causes charges to get accumulated to two ends of the needle-like fibres and an effective electrostatic interaction causes such peculiar exhibition. Other interesting possibility is that n-TSI is a ‘ferroelectric’ metal similar to the polar metal $LiOsO_3$ [1-3].

**Section S1.1: Structural Characterization:** Through single-crystal XRD studies, we find that the material crystallizes in a non-centrosymmetric tetragonal structure (space group $P\text{-}42_1c$, no. 114) with empirical formula $(TaSe_4)_3I$.

Single crystals were coated with Parabar oil and data were collected on a Bruker D8 VENTURE Microfocus diffractometer equipped with PHOTON II Detector, with Mo Kα radiation ($\lambda = 0.71073$ Å), controlled by the APEX III (v2017.3−0) software package. The raw data were integrated and corrected for Lorentz and polarization effects with the aid of the Bruker APEX III program suite. Absorption corrections were performed by using SADABS. Space groups were assigned by considering the systematic absences (determined by XPREP) and analysis of metric symmetry. Space groups were further checked by PLATON [4-5] for additional symmetry. The structure was solved by direct methods and refined against all data in the reported 2θ ranges by full-matrix least-squares refinement on F2 using the SHELXL [6] program suite and the OLEX2 [7] interface.

***Table S1:*** *$(TaSe_4)_3I$ structural information*

| Sample | **$(TaSe_4)_3I$** |
|---|---|
| Temperature | **T = 100 K** |
| Crystal system | Tetragonal |
| Space Group | P-4$2_1$c (no 114) |
| Lattice parameters | a = b = 9.436(5) Å<br>c= 19.046(11) Å<br>$\alpha = \beta = \gamma = 90^0$ |
| Unit cell volume (Å$^3$) | 1695.78 |
| R factor | 2.27% |

n-TSI is a member of linear chain compounds, namely, transition metal tetrachalco-halogenides (TMTCH) with generic formula $(MX_4)_nY$ where M = transition metal like Nb, Ta; X = chalcogen like S, Se; Y = halogen like Br, I and the constant n = 2, 3, 10/3. Typical optical image (Figure S2. a) and field emission scanning electron microscopy (FESEM, Zeiss Sigma) images (Figure S2b-c) show fibre like structure of n-TSI. Quasi-1D structure is also obvious from distinct lattice chain in the transmission electron microscopy (TEM using FEI, TECNAI G$^2$ F30, S-Twin microscope) images (Figure S3a-b). Schematics in Figures S3c and S3d show the lattice structure projected onto the *ab*-plane and *ca*-plane, respectively. Each individual chain is built of $TaSe_4$ antiprism (alternatively, the repeat unit of $TaSe_4$ can also be considered as two edge-connected tetrahedrons or two base-connected rectangular pyramids), stacked along the tetragonal *c*-axis into chains in a screw-like arrangement (Figure S3e). Parallel $TaSe_4$ chains are separated by iodine atoms. The strength of the bonding along the chain is quite strong whereas the interaction between parallel chains is van der Waals type and that is why the material can be exfoliated as 2D layers parallel to *ca*-plane or *cb*-plane. The structure being tetragonal and the basis *a* and *b* are equivalent. Breaking of inversion symmetry through just a small difference in relative position and spacing of iodine makes n-TSI unique in the TMTCH family and in particular, completely different from its centrosymmetric counterpart, c-TSI (simple tetragonal, space group P4/mnc, no. 128; semiconductor with no magnetic ordering and no superconductivity) with respect to the electronic properties. Lack of inversion symmetry is likely to change the internal electronic environment, for example, some otherwise vanishing components of local electric field may survive now. The lattice parameters of n-TSI are $a = b$ = 9.4358(5) Å; $c$ = 19.0464(11) Å and the angles are $\alpha = \beta = \gamma = 90^0$ (detailed information regarding the crystal structure is available in the Cambridge Crystallographic Data Centre (CCDC #2055811). There are six Ta-atoms along each $TaSe_4$ chain in a unit cell. The metal

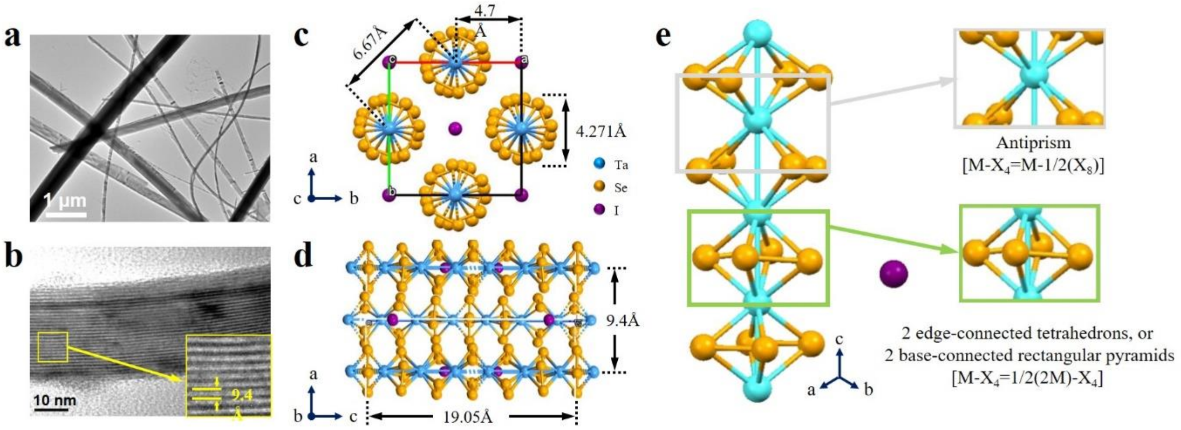


***Figure S3:*** *(a-b) Transmission electron microscopy (TEM) images showing belt like fibres and parallel linear chains in hi-resolution image, respectively. (c-d) Schematic of the lattice structure projected onto the ab- and ca-plane, respectively. (e) Each individual chain is built of* $TaSe_4$ *antiprism (alternatively, the repeat unit of* $TaSe_4$ *can also be considered as two edge-connected tetrahedrons or two base-connected rectangular pyramids), stacked along the tetragonal c-axis into chains in a screw-like arrangement.*

bonding sequence along a chain is the repetition of [-- long (3.306 Å) – intermediate (3.116 Å) -- short (3.051 Å)] bonds. In the Supplementary Figure S3. (c-d), it is obvious that the inter-chain separation in the *ca*-plane (*i.e.*, along the basis vectors *a* or *b*) is ~ 9.4Å (the shortest inter-chain separation is $9.4/\sqrt{2} = 6.67$ Å and the diameter of each $TaSe_4$ chain is 4.271Å. The shortest distance between I-atom and Se-atom is 3.236 Å.

**<u>Section S1.2</u>: XPS studies:** The conventional surface electron picture has been confirmed by X-ray photo-emission spectroscopy (XPS) [8] with an Al $K_\alpha$ monochromatic source (energy resolution is 0.5 eV). These measurements were performed with an OMICRON electron spectrometer, equipped with a SCIENTA OMICRON SPHERA analyser. The Figure S4 (a-d) shows the high-resolution XPS spectra for n-TSI. The binding energies of Ta-$4f_{7/2}$ (23.72 ± 0.05 eV) and Ta-$4f_{5/2}$ (25.65 ± 0.05 eV) gave the evidence of the existence in 4f electron state. Ta 4f region has well separated spin-orbit components ($D_{metal}$ = 1.93 ± 0.05 eV). The presence of I in n-TSI was confirmed from the peak position at 630.52 ± 0.05 eV (I $3d_{3/2}$) and 619.00 ± 0.05 eV (I $3d_{5/2}$). Se 3d peak was fitted with doublet peak as the peak has overlapping spin-orbit components (D = 0.87 ± 0.05 eV). From valence band data the density of states near the Fermi level proves the metallicity of n-TSI at room temperature. By calculation the area under

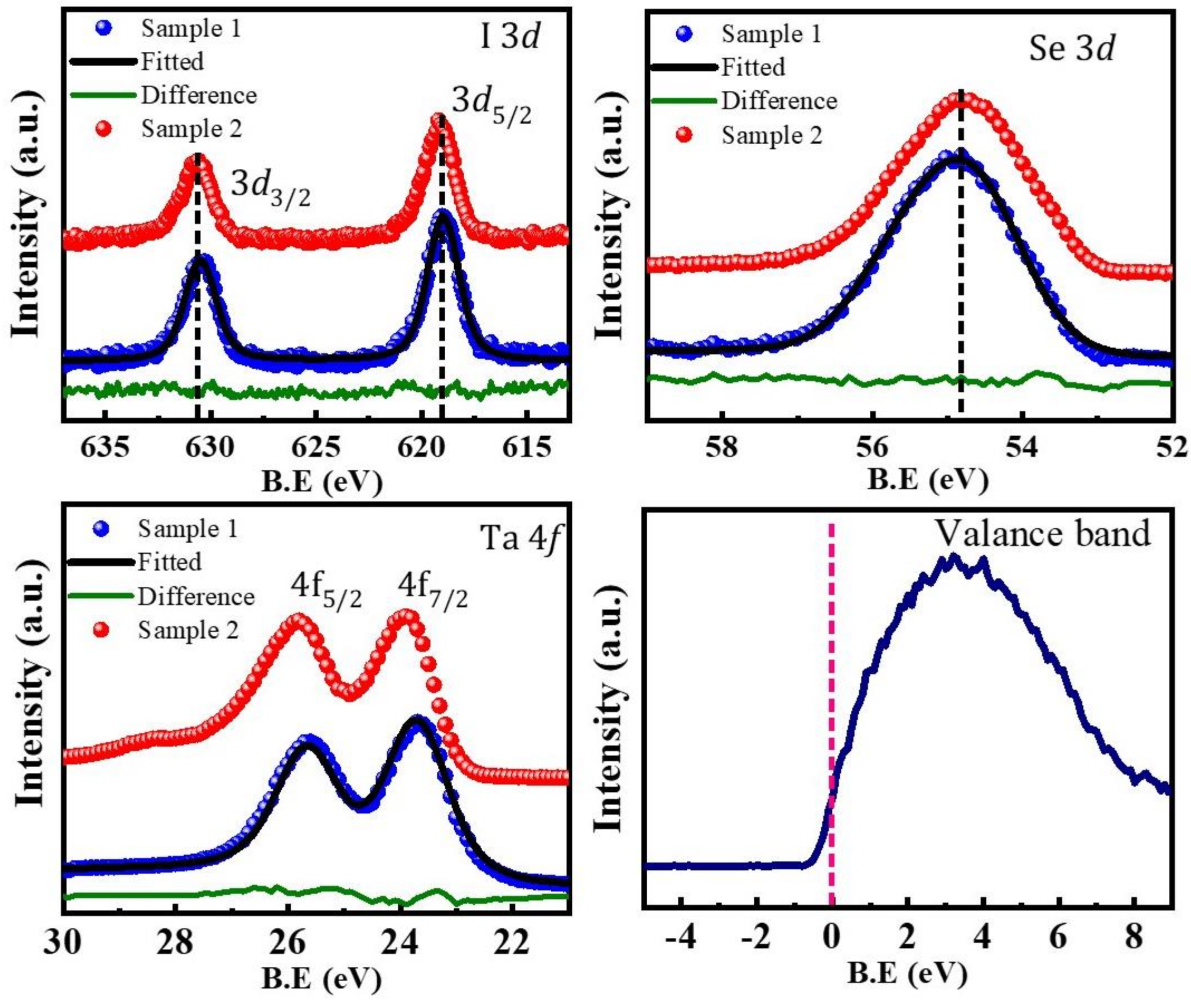


***Figure S4:*** *(a) The presence of I in n-TSI was confirmed from the peak position at 630.52 ± 0.05 eV (I $3d_{3/2}$) and 619.00 ± 0.05 eV (I $3d_{5/2}$). (b) Se 3d peak was fitted with doublet peak as the peak has overlapping spin-orbit components (D = 0.87 ± 0.05 eV). (c) The binding energies of Ta-$4f_{7/2}$ (23.72 ± 0.05 eV) and Ta-$4f_{5/2}$ (25.65 ± 0.05 eV) gave the evidence of existence in 4f electron state. Ta 4f region has well separated spin-orbit components ($D_{metal}$ = 1.93 ± 0.05 eV). (d) From valence band data the density of states near the Fermi level proves the metallicity of n-TSI at room temperature.*

the peak of Ta 4f, Se 3d and I 3d we got the stoichiometric ratio of Ta: Se: I = 3.01: 11.97: 1, which matches with the theoretical stoichiometry.

**<u>Section S2.1</u>: Transport measurement in a single ribbon n-TSI device:** We have also observed the superconducting transition at $T_c^{onset}$ ~ 2.6 K (Figure S5a, upper inset) and zero resistance state was achieved below 2 K in a single ribbon n-TSI sample with an average width ~ 900 nm (Sample Id - SWD1, Table S2). Here, we made four contacts (Figure S5a, bottom inset) using silver paint (RS components) for performing four-terminal transport measurements in PPMS DynaCool (QD) system. Figure S5b shows the temperature-dependent I-V characteristics from superconducting state (1.7K) to normal state (3K), measured in four-terminal geometry. These I-V characteristics are found to be non-linear with the critical current $I_c$ ~ 0.12mA. The analysis of detail I-V measurements are ongoing and will be communicated separately.

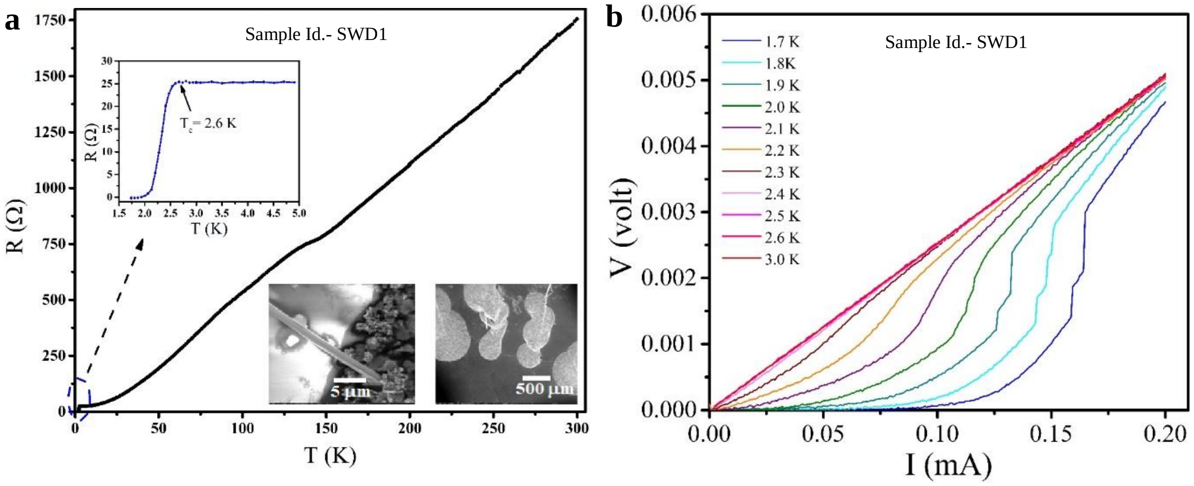


***Figure S5:*** *(a) Temperature-dependent four-terminal resistance of a single ribbon sample. (Upper inset) Superconducting transition and (bottom inset) SEM image of single ribbon and its four-terminal contacts. (b) Temperature-dependent I-V characteristics.*

## <u>Section S2.2</u>: Additional transport data from different samples

4 probe resistivity measurement was performed on several devices (bulk to single ribbon). Details of the measured devices are shown in Table S2 and additional temperature dependent transport data are shown in Figure S6a-d. In the main manuscript, we provide detail characterization from Device 2.

***Table S2****: Details of the devices*

| Device Name | Type | Observations |
|---|---|---|
| **FWD1** | Few wire | CDW |
| **FWD2** | Few wire | CDW, Superconductivity |

| | | |
|---|---|---|
| **FWD3** | Few wire | CDW |
| **BD1** | Bulk | CDW |
| **SWD1** | Single wire | CDW, Superconductivity |

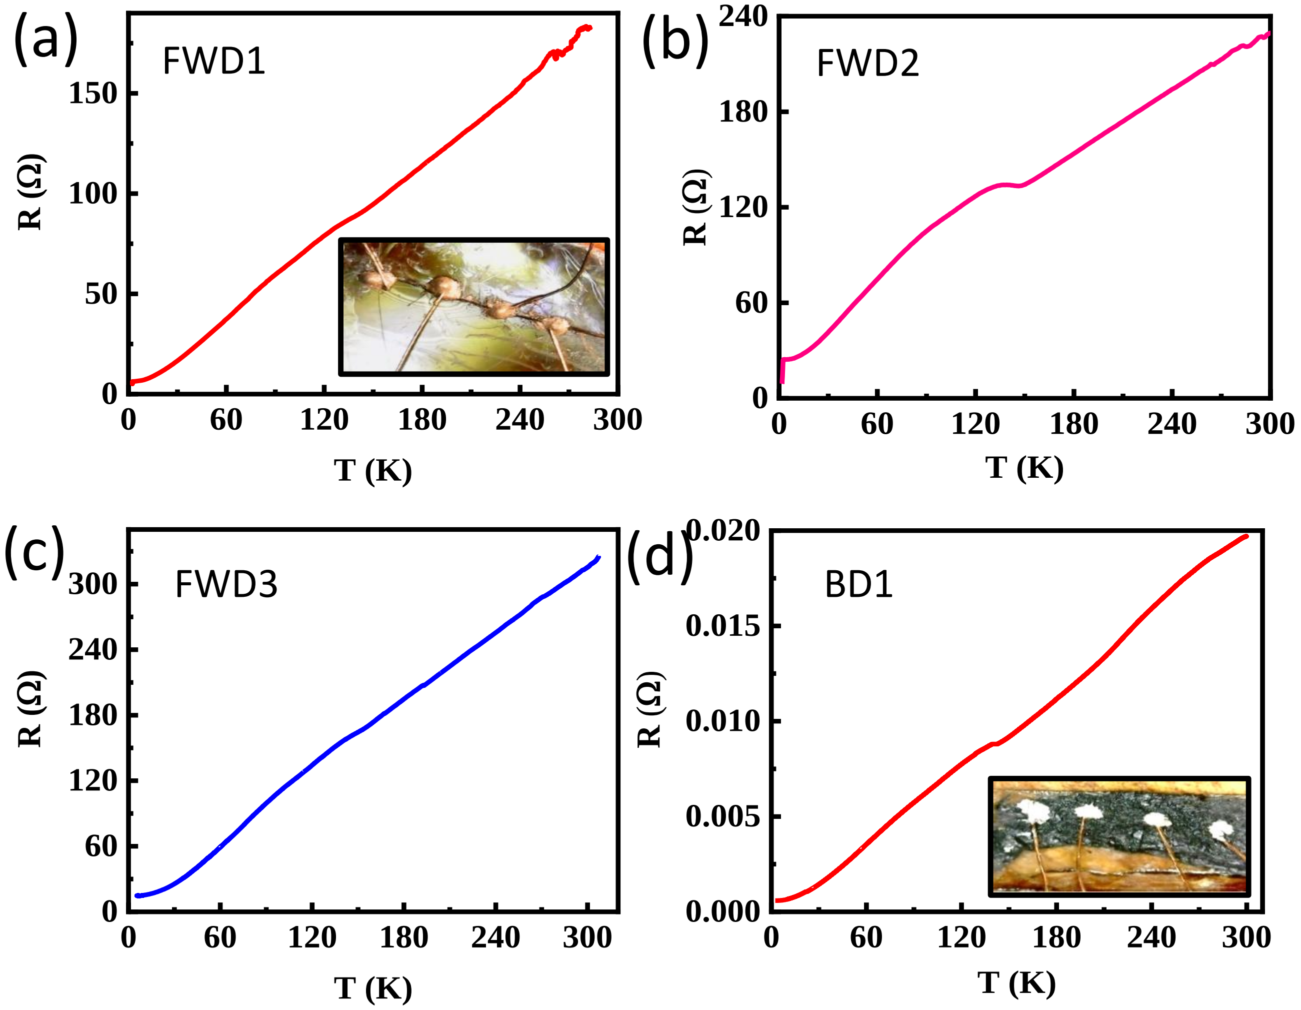


***Figure S6:*** *Low temperature transport measurement for different devices/wire shows metallic in nature with strong signature of CDW transition at around 150 K.*

## Section S3: Anisotropic electronic and magnetic properties:

### Section S3.1: Temperature-dependent and angle-dependent magneto-transport

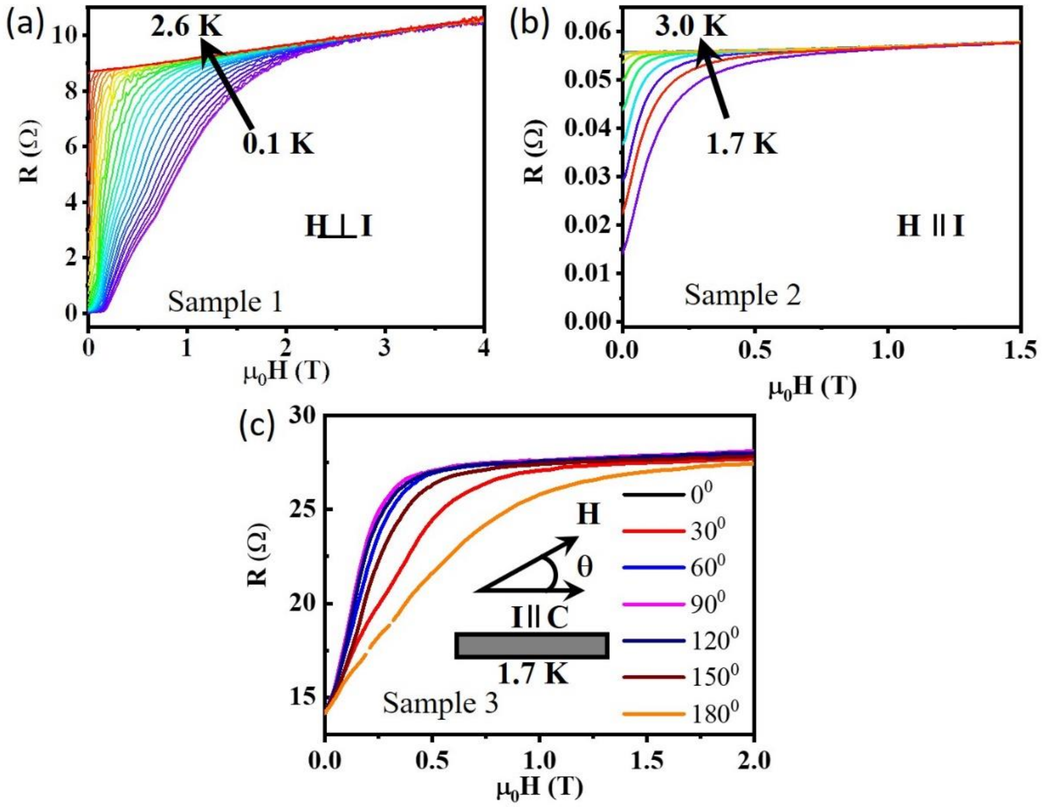


***Figure S7:*** *Temperature-dependent magneto-resistance of n-TSI with the magnetic field applied (a) perpendicular to current, (b) parallel to current. (c) Magneto-resistance with different oblique angles at T = 1.7K.*

We performed resistance vs magnetic field (R-B) measurements (of different samples) at different temperatures (from 0.1K to 2.6K) in the Dilution Refrigerator (Oxford Instruments) with magnetic field applied perpendicular to the current direction (Figure S7. (a)). Also, the same from 1.7K to 3.0K in PPMS DynaCool (QD) system with magnetic field applied parallel to the current direction (Figure S7. (b)). The Figure S7. (c) shows the anisotropy of the sample in the superconducting state.

**Section S3.2: Anisotropy in two-coil measurement with rotating magnetic field:** We carried out field-angle dependent mutual inductance measurement inside a superconducting vector magnet to resolve the anisotropic magnetic response in the superconducting phase. As shown in Figure S8, the secondary pick-up signal at 20 mT shows a clear two-fold symmetry when the magnetic field is rotated in the plane of the ribbon. A similar anisotropy is also seen in the field-angle dependent magnetoresistance measurement (Figure S7). These observations strongly suggest that the magnetic response of the superconducting phase is highly anisotropic. The observed anisotropy in the magnetic response discussed above may also arise from an anisotropy of the critical field alone, and not from an unconventional (non-BCS) pairing mechanism.

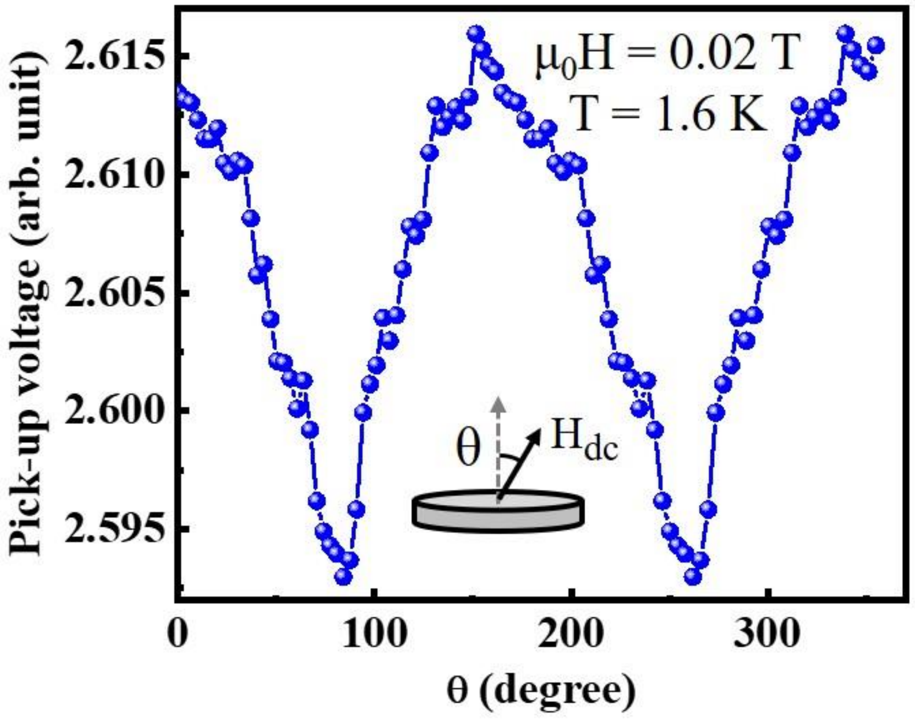


***Figure S8:*** *Field-angle dependent mutual inductance measurement inside a super- conducting vector magnet shows a twofold symmetry of the superconducting state.*

# <u>Section S4</u>: Magnetization data at low temperatures

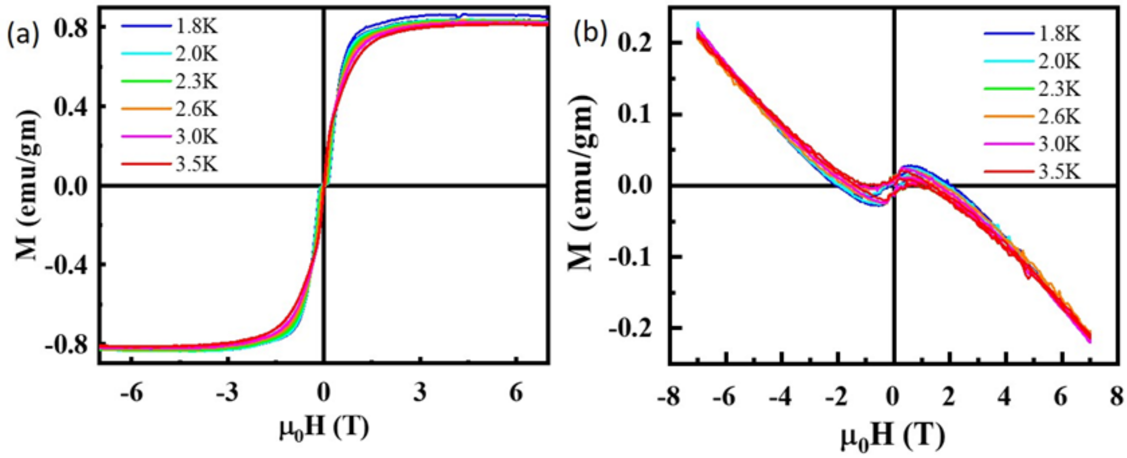


***Figure S9:*** *Raw magnetization measurement in n-TSI. (a-b) observation of S shape loop in MH data parallel to the c and ab directions. In parallel to ab direction, the MH data shows a significant diamagnetic contribution from GE varnish as seen in b.*

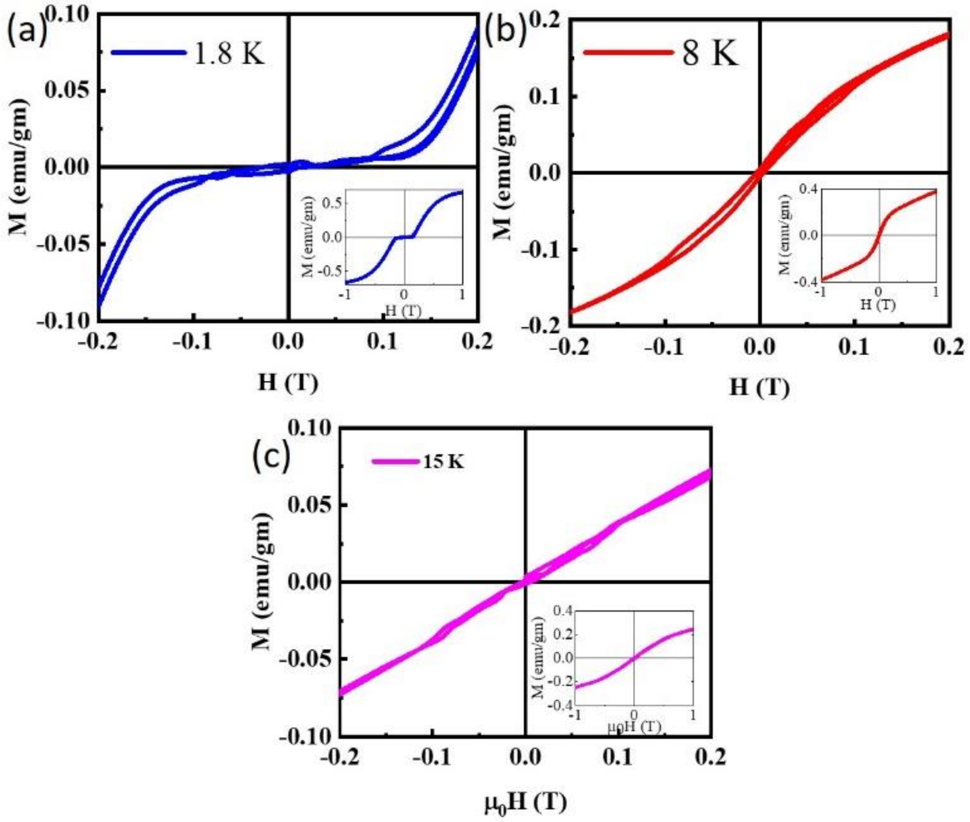


***Figure S10:*** *Raw magnetization measurement in n-TSI parallel to c axis at temperature (a) below superconducting transition (T<Tc), (b) below magnetic transition and above the superconducting transition ((Tc<T<Tm) (c) above the magnetic transition (T>Tm>Tc).*

To probe the magnetic ordering, we concentrate on MH measurement. A typical '**S'** shaped loop has been observed parallel to c-direction of the sample. The low temperature and low filed data in this direction show some interesting feature due to superconductivity which is discussed in detailed in the main paper. Now for the ab direction data we can see a strong diamagnetic contribution due to the GE varnish affecting the MH loop. To correct the diamagnetic contribution, we have assumed saturated magnetization to be the same in both direction and a paramagnetic fitting was done to correct the data. Figure S10. (a) shows a flat region which is originated due to the Meissner effect from the SC phase, at T = 1.8K. MH loops at different temperatures (Figure S10. a-c) indicate the coexistence of superconductivity and ferromagnetic phase in n-TSI at $T<T_c$.

## Section S5: Estimation of transition temperature of superconducting phase ($T_{SC}$) and Ferromagnetic phase ($T^*_m$) from MT data:

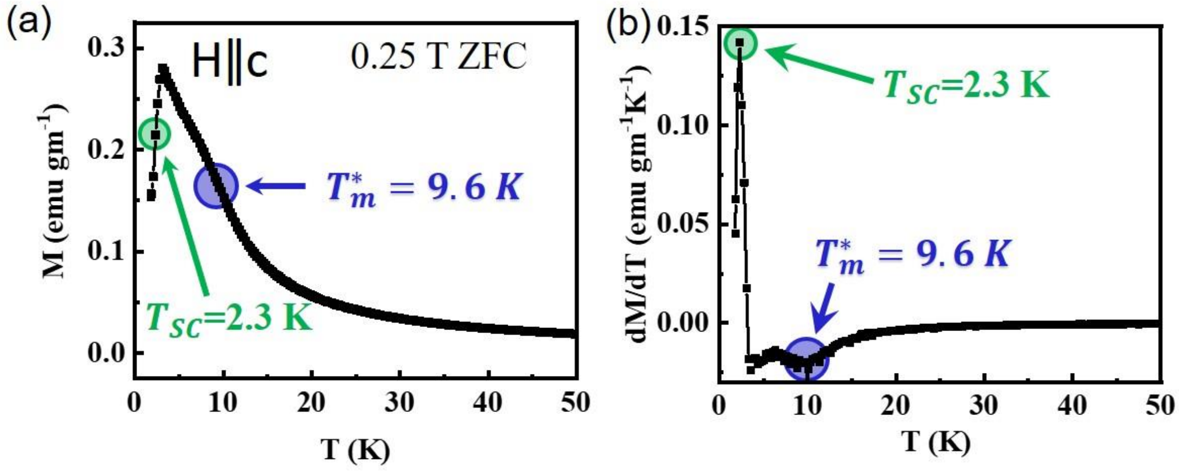


***Figure S11:*** *(a) ZFC MT data at applied field 0.25 T parallel to c axis and (b) corresponding dM/dT vs. T plot. The superconducting transition temperature is estimated when M shows a sudden drop due to Meissner effect (or peak in the dM/dT vs. T plot as shown in panel b) and paramagnet to ferro magnet transition temperature where M shows the signature of magnetic ordering (or dip in the dM/dT vs T plot).*

Figure S12 shows the temperature dependent inverse susceptibility ($1/\chi$) calculated from the MT data at applied magnetic field 0.25 T and its corresponding Curie-Weiss fit using the following equation,

$$C/\chi = T\text{-}T_{C\text{-}W} \ldots\ldots\ldots\ldots\ldots\ldots\ldots\ldots\ \ldots\ldots\ldots \quad \text{(i)}$$

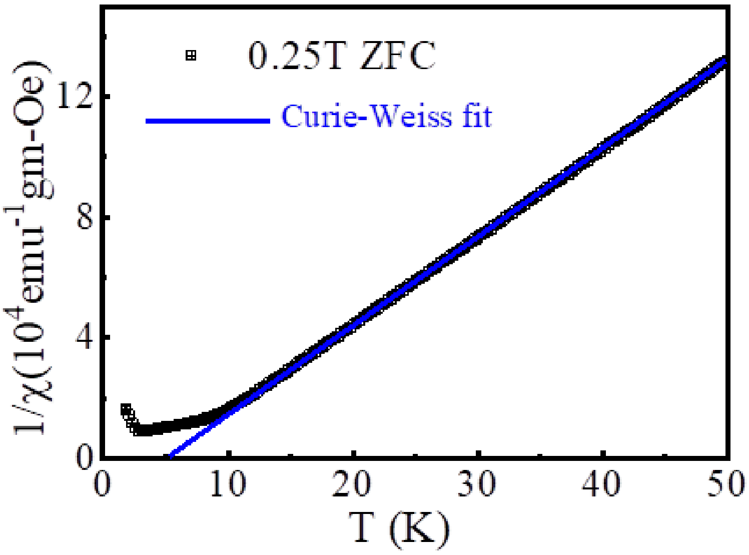


***Figure S12:*** *Temperature-dependent inverse susceptibility (1/c) parallel to the c axis under ZFC and warming at 0.25 T. The blue solid line is the fitted plot according to the Curie-Weiss law.*

Here, *C* is a material-specific Curie constant, *T* is the absolute temperature, and $T_{C\text{-}W}$ is the Curie- Weiss temperature. The estimated $T_{C\text{-}W}$ from the above fit is ~ 5.5 K which indicates the ferromagnetic ordering in the system at low temperature.

## Bibliography:


1. Anderson, P. W. & Blount, E. I. *Symmetry considerations on martensitic transformations: 'Ferroelectric' metals?* Phys. Rev. Lett. **14**, 217–219 (1965).

2. Shi, Y. *et. al. A ferroelectric-like structural transition in a metal.* Nature Materials **12**, 1024 (2013).

3. Berger, E. *et. al. Direct observation of symmetry-breaking in a 'ferroelectric' polar metal.* arXiv:2010.03134v4 (2020).

4. Spek, A. L. *Single-crystal structure validation with the program PLATON*. J. Appl. Crystallogr. **36**, 7-13 (2003).

5. Spek, A. L. *Structure validation in chemical crystallography*. Acta Crystallographica Section D **65**, 148-155 (2009).

6. Sheldrick, G. M. *A short history of SHELX*. Acta Crystallographica Section A **64**, 112-122 (2008).

7. Dolomanov, O. V. Bourhis, L. J. Gildea, R. J. Howard, J. A. K. Puschmann, H. *OLEX2: a complete structure solution, refinement and analysis program*. J. Appl. Crystallogr. **42**, 339-341 (2009).

8. Moulder, J. F. Stickle W. F. Sobol, P. E. Bomben, K. D. *Handbook of X Ray Photoelectron Spectroscopy: A Reference Book of Standard Spectra for Identification and Interpretation of XPS Data.* Physical Electronics Division, Perkin-Elmer Corporation, (1992).
